# Supplementary material for: Pairwise Fairness for Ordinal Regression
Source: arXiv:2105.03153 source file (2022-02-11)
Supplement: Supplementary file 1 [file appendix_convergence.tex]

\subsection{Convergence of $\Fairviol(f;\mathcal{D})$ to $\Fairviol(f;\Psymb)$}\label{appendix_convergnce}

We only consider the case that $\Fairviol=\DPviol$. The case $\Fairviol=\EOviol$ can be treated in an analogous~way.

It is not hard to see that 
    \begin{align*}
        |\DPviol(f;\Psymb)-\DPviol(f;\mathcal{D})|\leq 
        2 \max_{\tilde{a},\hat{a}\in\mathcal{A}}|\Psymb[f(x_1)> f(x_2) | a_1=\tilde{a},a_2=\hat{a}]-\widehat{\Psymb}_n[f(x_1)> f(x_2) | a_1=\tilde{a},a_2=\hat{a}]|, 
    \end{align*}
    where $\widehat{\Psymb}_n$ is the empirical distribution on $\mathcal{D}$, which is an i.i.d. sample from $\Psymb$, and $(x_1,y_1,a_1)$, $(x_2,y_2,a_2)$ are independent samples from $\Psymb$ and $\widehat{\Psymb}_n$, respectively. Let  $\mathcal{D}=((x_i,y_i,a_i))_{i=1}^n$ and fix $\tilde{a},\hat{a}$. Then 
\begin{align*}
	\widehat{\Psymb}_n[f(x_1)> f(x_2) | a_1=\tilde{a},a_2=\hat{a}]=\frac{
		\sum_{i,j\in[n]}
		\charfct[f(x_i)>f(x_j),a_i=\tilde{a},a_j=\hat{a}]}{
		\sum_{i,j\in[n]} \charfct[a_i=\tilde{a},a_j=\hat{a}]}.
\end{align*}

The random variables $\charfct[f(x_i)>f(x_j),a_i=\tilde{a},a_j=\hat{a}]_{i,j\in[n]}$ are a read-$n$ family \citep[][Definition~1]{gavinsky_tail_bound}. It is $\Psymb[\charfct[f(x_i)>f(x_j),a_i=\tilde{a},a_j=\hat{a}]=1]=\Psymb[f(x_i)>f(x_j),a_i=\tilde{a},a_j=\hat{a}]$ for $i\neq j$ and $\Psymb[\charfct[f(x_i)>f(x_j),a_i=\tilde{a},a_j=\hat{a}]=1]=0$ for $i=j$. 
It follows from  
\cite[Theorem 1.1]
{gavinsky_tail_bound} that for any $\varepsilon>0$,  
with 
probability $1-2e^{-2\varepsilon^2n}$ over the sample $\mathcal{D}$ we have
\begin{align*}
	\frac{\sum_{i,j\in[n]}\charfct[f(x_i)>f(x_j),a_i=\tilde{a},a_j=\hat{a}]}{n^2}
	\leq \Psymb[f(x_1)>f(x_2),a_1=\tilde{a},a_2=\hat{a}]+\varepsilon
\end{align*}
as well as 
\begin{align*}
	\frac{\sum_{i,j\in[n]}\charfct[f(x_i)>f(x_j),a_i=\tilde{a},a_j=\hat{a}]}{n^2}\geq \Psymb[f(x_1)>f(x_2),a_1=\tilde{a},a_2=\hat{a}]-\frac{1}{n}-\varepsilon.
\end{align*}
Similarly, we have with 
probability $1-2e^{-2\varepsilon^2n}$ over the sample $\mathcal{D}$ that 
\begin{align*}
\Psymb[a_1=\tilde{a},a_2=\hat{a}]-\varepsilon -\frac{1}{n}\leq 	\frac{\sum_{i,j\in[n]}\charfct[a_i=\tilde{a},a_j=\hat{a}]}{n^2}
	\leq \Psymb[a_1=\tilde{a},a_2=\hat{a}]+\varepsilon.
\end{align*}
It follows that if $\Psymb[a_i=\tilde{a},a_j=\hat{a}]$ is lower bounded by some positive constant, for any $\delta>0$, with 
probability $1-\delta$ over the sample $\mathcal{D}$ we have
\begin{align*}
    |\Psymb[f(x_1)> f(x_2) | a_1=\tilde{a},a_2=\hat{a}]-\widehat{\Psymb}_n[f(x_1)> f(x_2) | a_1=\tilde{a},a_2=\hat{a}]|\leq M \sqrt{\frac{\log\frac{1}{\delta}}{n}}.
\end{align*}
for some constant~$M$.  
This implies that with 
probability $1-\delta$  over the sample $\mathcal{D}$ we have
\begin{align*}
    \max_{\tilde{a},\hat{a}\in\mathcal{A}}|\Psymb[f(x_1)> f(x_2) | a_1=\tilde{a},a_2=\hat{a}]-\widehat{\Psymb}_n[f(x_1)> f(x_2) | a_1=\tilde{a},a_2=\hat{a}]|\leq M \sqrt{\frac{\log\frac{|\mathcal{A}|^2}{\delta}}{n}}.
\end{align*}
